# Supplementary material for: Parity Push Post-Selection with Soft Parity Constraints for Quantum LDPC Codes
Source: arXiv:2611.23759 source file (2026-11-18)
Supplement: Supplementary file 1 [file si_setup.tex]

\makeatletter\if@twocolumn\onecolumn\fi\makeatother   
\setcounter{figure}{0}
\setcounter{table}{0}
\setcounter{equation}{0}
\renewcommand{\theHtable}{S\arabic{table}}
\renewcommand{\theHfigure}{S\arabic{figure}}
\renewcommand{\figurename}{Supplementary Figure}
\renewcommand{\tablename}{Supplementary Table}
\renewcommand{\theequation}{S\arabic{equation}}
\newcounter{snote}
\newcommand{\snote}[2]{\refstepcounter{snote}%
  \section*{Supplementary Note \thesnote: #1}\label{#2}}
\newcommand{\sifig}[2][\textwidth]{%
  \IfFileExists{figures/#2}{\includegraphics[width=#1]{#2}}{%
    \fbox{\parbox[c][0.3\textheight][c]{\dimexpr#1-2\fboxsep-2\fboxrule\relax}{\centering\ttfamily \detokenize{#2}\\[2pt](figure not yet generated)}}}}
\makeatletter
\setlength{\@fptop}{0pt}
\setlength{\@fpsep}{12pt plus 1fil}
\setlength{\@fpbot}{0pt plus 1fil}
\makeatother
